# Supplementary material for: Non-Zhang-Rice singlet character of the first ionization state of T-CuO
Source: arXiv:1602.01113 source file (2016-02-02)
Supplement: Supplementary file 1 [file supplement.pdf]

# Supplemental Material for "Non-Zhang-Rice singlet character of the first ionization state of T-CuO"

Clemens P.J. Adolphs, Simon Moser, George A. Sawatzky, and Mona Berciu
(Dated: October 27, 2015)

## HAMILTONIAN - TECHNICAL DETAILS

For simplicity of notation, we provide here the explicit expressions for the terms in the $CuO_2$ Hamiltonian, assuming that only the ligand O $2p$ orbitals are included. Generalization to including both sets of O $2p$ orbitals, and also to T-CuO, is straightforward.

With the sign of positive/negative lobs as pictured in Fig. 1 of the main article, and using $p^\dagger_{i,\sigma}$ as the creation operator for a hole in the ligand O $2p$ orbital located at $i$, we have:

$$T_{pp} = t_{pp} \sum_{i\in \mathrm{O},\boldsymbol{\delta},\sigma} r_{\boldsymbol{\delta}} p^\dagger_{i,\sigma} p_{i+\boldsymbol{\delta},\sigma} - t'_{pp} \sum_{i\in \mathrm{O},\sigma} p^\dagger_{i,\sigma}(p_{i-\boldsymbol{\epsilon},\sigma} + p_{i+\boldsymbol{\epsilon},\sigma}).$$

The lattice constant is set to $a = 1$. The vectors $\boldsymbol{\delta} = \pm(0.5, 0.5), \pm(0.5, -0.5)$ are the distances between any O and its four nn O sites, and $r_{\boldsymbol{\delta}} = \pm 1$ sets the sign of each nn $pp$ hopping integral in accordance with the overlap of the $2p$ orbitals involved. Next nn hopping is included only between O $2p$ orbitals pointing toward a common bridging Cu, separated by $\boldsymbol{\varepsilon} = (1, 0)$ or $(0, 1)$; hybridization with the $4s$ orbital of the bridging Cu further boosts the value of this hopping integral.

The spin-swapping hopping term is:

$$T_{\mathrm{swap}} = -t_{sw} \sum_{i\in \mathrm{Cu},\mathbf{u}\neq\mathbf{u}'} \sum_{\sigma,\sigma'} s_{\mathbf{u}-\mathbf{u}'} p^\dagger_{i+\mathbf{u},\sigma} p_{i+\mathbf{u}',\sigma'} |i_{\sigma'}\rangle\langle i_\sigma|,$$

where $\mathbf{u}, \mathbf{u}' = (\pm 0.5, 0), (0, \pm 0.5)$ are the distances between a Cu and its four nn O sites. This term shows the change of the Cu spin located at $\mathbf{R}_i$ from $\sigma$ to $\sigma'$ as the doped hole changes its spin from $\sigma'$ to $\sigma$ while moving to another O. The sign $s_{\boldsymbol{\eta}} = \pm 1$ is due to the overlaps of the $2p$ and $3d$ orbitals involved in the process, and the overall minus in front is because of the interchange in the order of the two holes (which is on O and which is on Cu).

The Cu-Cu AFM superexchange is the usual:

$$\hat{H}_{J_{dd}} = J_{dd} \sum_{\langle i,j\rangle'} \mathbf{S}_i \cdot \mathbf{S}_j,$$

where $\mathbf{S}_i$ is the Cu spin at site $i$ and the sum runs over all nearest-neighbor pairs except the one that has the doping hole on their bridging O. Finally,

$$\mathcal{H}_{J_{pd}} = J_{pd} \sum_{i,\mathbf{u}} \mathbf{s}_i \cdot \mathbf{S}_{i+\mathbf{u}}$$

is the exchange of the hole's spin $\mathbf{s}_i = \frac{1}{2}\sum_{\alpha,\beta} p^\dagger_{i\alpha} \boldsymbol{\sigma}_{\alpha\beta} p_{i\beta}$ with its two nn Cu spins.

## VARIATIONAL METHOD

For any given momentum $\mathbf{k}$, our corresponding variational Hilbert space contains all states with at most $n_m$ magnons and with a restriction on the maximum allowed magnon-hole distances, as discussed next.

Zero-magnons states are the eight Bloch states of momentum $\mathbf{k}$, one for each of the eight oxygen orbitals in the magnetic unit cell. States with magnons are Bloch states of total momentum $\mathbf{k}$ for given hole and magnons configurations with fixed relative distances between holes and magnons. For example, the one-magnon states have the form

$$|\mathbf{k}, \alpha, \boldsymbol{\delta}\rangle = \frac{1}{\sqrt{N}} \sum_i e^{i\mathbf{k}\cdot\mathbf{r}_i} p^\dagger_{i\alpha,\downarrow} S^+_{i+\boldsymbol{\delta}} |\text{Néel}\rangle$$

where $i$ runs over the unit cells, $i\alpha$ denotes oxygen orbital $\alpha = 1, \ldots, 8$ within unit cell $i$, and $S^+_{i+\boldsymbol{\delta}}$ is the magnon creation operator for a down-spin copper of the magnetic unit cell located a distance $\boldsymbol{\delta}$ away from unit cell $i$. The two-magnon and three-magnon states are constructed similarly by adding magnons in the units cells located at distances $\boldsymbol{\delta}_2$ and $\boldsymbol{\delta}_3$ apart, respectively.

Our restriction is that any $|\boldsymbol{\delta}| \leq N_{\max}$. For the 1- and 2-magnon states, the variational approach together with the Lanczos method can easily handle distances of up to $N_{\max} = 10$, although the low-energy (quasiparticle) results are converged even for $N_{\max} = 2$. This is not surprising because we are concerned with the physics of the polaronic bound state, where the magnons are bound close to the hole. For the 3-magnon states, we set $N_{\max} = 1$, *i.e.* we only include 3-magnon configurations where the 3 magnons are located either in the same unit cell as the hole, or in a unit cell directly adjacent to it. These are the configurations with the highest weight in the quasiparticle cloud but, as the results show, they do not lead to significant changes. Less likely 3-magnon configurations, with the magnons spread farther apart, can therefore be safely ignored at these energies.

We note that this approximation is valid for calculating low-energy properties. It would fail at describing higher energy features such as the correct locations for the polaron+one-magnon continuum, since its states necessarily have a magnon far away from the polaron, so

the corresponding configurations need to be included to capture such higher energy features.

The resulting Hamiltonian matrix in this basis is sparse: for each configuration, there are only a few allowed hoppings and spin flips. Thus, it readily lends itself to the Lanczos method, which provides us with the spectral function $A(\mathbf{k},\omega)$ relying only on computationally cheap matrix-vector products. The lowest-lying peak in the spectral function then gives us the $qp$ dispersion.

## ZHANG-RICE SINGLET BLOCH STATE

For the $CuO_2$ lattice, taking into consideration the AFM order of the Cu spins, we can choose the unit cell as shown in Fig. 1(a), with the corresponding magnetic Brillouin zone shown in Fig. 1(b).

To define a ZRS Bloch state, we first introduce:

$$p^\dagger_{x^2-y^2,i,\sigma} = \frac{1}{2}\left[p^\dagger_{i+\frac{\mathbf{x}}{2},\sigma} + p^\dagger_{i+\frac{\mathbf{y}}{2},\sigma} - p^\dagger_{i-\frac{\mathbf{x}}{2},\sigma} - p^\dagger_{i-\frac{\mathbf{y}}{2},\sigma}\right]$$

which describes the doped hole occupying a linear combination of ligand orbitals with $x^2-y^2$ symmetry, centered on the Cu located at $i$. The ZRS is obtained when a hole occupying such a state is locked in a singlet with the Cu spin, therefore a ZRS Bloch state can be defined as:

$$|d,\mathbf{k}\rangle = \sum_{i\in \mathrm{Cu}_\downarrow} \frac{e^{i\mathbf{k}\cdot\mathbf{R}_i}}{\sqrt{N}} \frac{p^\dagger_{x^2-y^2,i,\uparrow} - p^\dagger_{x^2-y^2,i,\downarrow}S^+_i}{\sqrt{2}} |\mathrm{N}\rangle. \quad (1)$$

Here, $\mathbf{k}$ is any momentum in the magnetic Brillouin zone, the sum is only over sites in the spin-down Cu sublattice (since a spin-up doped hole can form a ZRS only with these spins), and $|\mathrm{N}\rangle$ is the Néel state.

Of course, one can also define Bloch states associated with singlets that have other symmetries for the linear

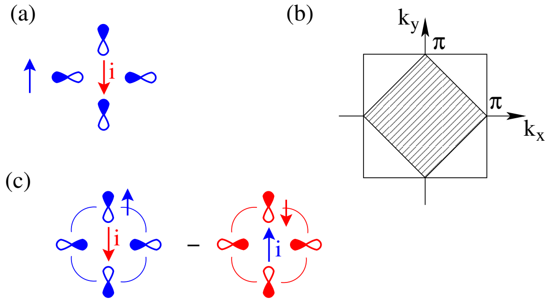


FIG. 1: (a) Unit cell for $CuO_2$, with two Cu spins and four ligand O orbitals. We use the location $i$ of the down-spin Cu as the reference point. The white/shaded areas indicate our choice for positive/negative lobs. (b) Magnetic Brillouin zone (shaded region) vs. full Brillouin zone (unshaded). (c) ZRS between a hole occupying the linear combination of ligand orbitals with $x^2-y^2$ symmetry, and the spin of the central Cu. The Bloch state is obtained from its translations on the corresponding magnetic sublattice.

combination of O orbitals. Of all these states, in $CuO_2$ the ZRS Bloch state is found to have the largest overlap with the low-energy quasiparticle wavefunction.

Its first excited state, on the other hand, is found to have the largest overlap with Bloch states based on the singlet with $x-y$ symmetry, *i.e.* the singlet obtained using $p^\dagger_{x-y,i,\sigma} = \frac{1}{2}\left[p^\dagger_{i+\frac{\mathbf{x}}{2},\sigma} + p^\dagger_{i+\frac{\mathbf{y}}{2},\sigma} + p^\dagger_{i-\frac{\mathbf{x}}{2},\sigma} + p^\dagger_{i-\frac{\mathbf{y}}{2},\sigma}\right]$ instead of $p^\dagger_{x^2-y^2,i,\sigma}$ in Eq. (1). We call this state $|p,\mathbf{k}\rangle$.

## LOW-ENERGY EFFECTIVE THEORY

As discussed above, the low-energy quasiparticle wavefunction for a $CuO_2$ layer has the largest overlap with the ZRS Bloch state with $x^2-y^2$ symmetry. For the T-CuO lattice, if we turn off the inter-sublattice hopping $\hat{T}_{mix}$, the doped hole is constrained to move on one set of $p$ orbitals and therefore interacts only with the Cu for which those orbitals are ligand. The resulting quasiparticle is exactly like for $CuO_2$, but in this case the eigenstate is doubly degenerate since the ZRS can live on either sublattice of ligand orbitals.

Previously, we have viewed T-CuO as two copies of a $CuO_2$ lattice, by adding two more Cu ions and four more oxygen orbitals to the unit cell while keeping the same lattice vectors. An alternative view is to use the same unit cell as for $CuO_2$, i.e., two copper ions and four oxygen orbitals, but have one of the lattice vectors shortened by a factor 2, depending on the relative magnetic ordering of the sublattices. If the copper spins are aligned ferromagnetically along the main diagonal, the proper lattice vectors are $\mathbf{a}_1 = a(1/2,1/2)^T$ and $\mathbf{a}_2 = a(-1,1)^T$.

While both views are valid, the latter view has the smallest possible unit cell and thus does not exhibit folding of the true Brillouin zone.

For a very simple effective theory, we use perturbation theory to investigate the influence of the inter-sublattice hopping $\hat{T}_{mix}$. Because this operator moves the hole between the two sets of O orbitals but cannot move magnons between the different Cu sublattices, only the magnon-free part of the quasi-particle wavefunction will contribute to matrix elements of this operator. Consider a two-dimensional Hilbert space containing the $d$- and $p$-wave ZRS states of momentum $\mathbf{k}$. Without $\hat{T}_{mix}$, we have

$$H = \begin{pmatrix} E_0 & 0 \\ 0 & E_1 \end{pmatrix}$$

where $E_0(\mathbf{k})$ and $E_1(\mathbf{k})$ are the $CuO_2$ dispersions of the groundstate and the first excited state.

We now apply $\hat{T}_{mix}$ to each of the four oxygen basis states from which the ZRS-type states are built. Let

$$|1,\mathbf{k}\rangle := \sum_{i\in \mathrm{Cu}_\downarrow} \frac{e^{i\mathbf{k}\cdot\mathbf{R}_i}}{\sqrt{N}} p^\dagger_{i+\frac{\mathbf{x}}{2},\uparrow}|N\rangle.$$

and $|2,\mathbf{k}\rangle$, $|3,\mathbf{k}\rangle$ and $|4,\mathbf{k}\rangle$ defined analogously for the other oxygen orbitals enumerated counter-clockwise around the same copper ion. Note that here the sum is over all down-spins in the T-CuO lattice. Taking care of the proper phases for the hoppings, we have

$$\hat{T}_{mix}|1,\mathbf{k}\rangle = -2\tilde{t}_{pp}\cos(\mathbf{k}\cdot\mathbf{a}_1)|1,\mathbf{k}\rangle - \tilde{t}_{pp}\left[e^{-i\mathbf{k}\cdot\mathbf{a}_1} + e^{-i\mathbf{k}\cdot(\mathbf{a}_1-\mathbf{a}_2)}\right]|3,\mathbf{k}\rangle$$
$$\hat{T}_{mix}|2,\mathbf{k}\rangle = -2\tilde{t}_{pp}\cos(\mathbf{k}\cdot\mathbf{a}_1)|2,\mathbf{k}\rangle - \tilde{t}_{pp}\left[e^{-i\mathbf{k}\cdot\mathbf{a}_1} + e^{-i\mathbf{k}\cdot(\mathbf{a}_1+\mathbf{a}_2)}\right]|4,\mathbf{k}\rangle$$
$$\hat{T}_{mix}|3,\mathbf{k}\rangle = -2\tilde{t}_{pp}\cos(\mathbf{k}\cdot\mathbf{a}_1)|3,\mathbf{k}\rangle - \tilde{t}_{pp}\left[e^{i\mathbf{k}\cdot\mathbf{a}_1} + e^{i\mathbf{k}\cdot(\mathbf{a}_1-\mathbf{a}_2)}\right]|1,\mathbf{k}\rangle$$
$$\hat{T}_{mix}|4,\mathbf{k}\rangle = -2\tilde{t}_{pp}\cos(\mathbf{k}\cdot\mathbf{a}_1)|4,\mathbf{k}\rangle - \tilde{t}_{pp}\left[e^{i\mathbf{k}\cdot\mathbf{a}_1} + e^{i\mathbf{k}\cdot(\mathbf{a}_1+\mathbf{a}_2)}\right]|2,\mathbf{k}\rangle$$

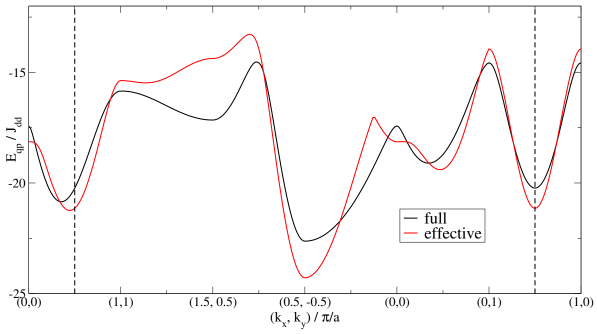


FIG. 2: Comparison between the one-magnon numerical dispersion and the effective calculations involving both the low-energy and first excited state quasiparticles. The results are in qualitative agreement, in particular the shift of the minimum along $k_x = k_y$. The dashed lines are a guide to the eye to demonstrate that the peak along $\Gamma - M$ gets shifted away from $\mathbf{k} = (\pi/2, \pi/2)$ yet remains there along $X - X'$.

From this, we can now compute $\langle d/p,\mathbf{k}|\hat{T}_{mix}|d/p,\mathbf{k}\rangle$.

$$\langle d,\mathbf{k}|\hat{T}_{mix}|d,\mathbf{k}\rangle = \tilde{t}_{pp}\cos(\mathbf{k}\cdot\mathbf{a}_1)\left[\cos(\mathbf{k}\cdot\mathbf{a}_2)-1\right]$$
$$\langle p,\mathbf{k}|\hat{T}_{mix}|p,\mathbf{k}\rangle = \tilde{t}_{pp}\cos(\mathbf{k}\cdot\mathbf{a}_1)\left[\cos(\mathbf{k}\cdot\mathbf{a}_2)-3\right]$$
$$\langle p,\mathbf{k}|\hat{T}_{mix}|d,\mathbf{k}\rangle = i\tilde{t}_{pp}\sin(\mathbf{k}\cdot\mathbf{a}_1)\left[\cos(\mathbf{k}\cdot\mathbf{a}_2)+1\right]$$

Strictly speaking, these matrix elements should be weighted by the appropriate quasiparticle weights $Z_\mathbf{k}$ corresponding to projection of the true *qp* eigenstate onto these non-interacting Bloch states. However, these weights are known to be rather featureless near the $(\pi/2, \pi/2)$ points that are most relevant in this discussion, so we ignore them in the following. This will affect results quantitatively, but not qualitatively.

It turns out that considering $\hat{T}_{mix}$ in this two-dimensional Hilbert space is already sufficient to explain qualitatively the quasi-particle physics of T-CuO.

Let us consider the special case of the $k_x = k_y = k$ line, where $\mathbf{k}\cdot\mathbf{a}_2 = 0$ and $\mathbf{k}\cdot\mathbf{a}_1 = ka$. We then have

$$T_{mix}(k) = \begin{pmatrix} 0 & -2i\tilde{t}_{pp}\sin(ka) \\ 2i\tilde{t}_{pp}\sin(ka) & -2\tilde{t}_{pp}\cos(ka). \end{pmatrix}$$

The numerical results showed that the minimum along this line gets shifted from $k = \pi/2$ closer to the $\Gamma$-point, and this readily follows from the simple form here: The off-diagonal elements provide mixing of the $d$- and $p$-states, and the energy $-2\tilde{t}_{pp}\cos(ka)$ of the $p$-state then moves the minimum to a lower $k$.

On the other hand, for $k_x = \pi - k_y = k$ we find that $T_{dd} = T_{pp} = 0$ and $T_{pd} = i\tilde{t}_{pp}\left[1+\cos(\pi-2k)\right]$. In this case, the Hamiltonian is symmetric around $k = \pi/2$, and thus the minimum gets only shifted down in energy while remaining at $k = \pi/2$. Other directions can be considered similarly.

In Fig. 2 we compare the full numerical results to the effective low-energy results from the $2\times 2$ Hamiltonian. The qualitative agreement is striking, in particular the shift of the minimum from $(\frac{\pi}{2}, \frac{\pi}{2})$ towards the $\Gamma$ point emerges as predicted. Of course, quantitative disagreements result from the crudeness of our approximation: we neglected the quasiparticle weights which would narrow the bandwidth for this effective low-energy result, we ignored other higher-energy eigenstates as well as the fact that the $CuO_2$ low-energy and first excited quasiparticles are not pure $x^2-y^2$- and $x-y$ ZRS-like Bloch states, respectively. Nonetheless, the results satisfactorily show that the changes near $(\frac{\pi}{2}, \frac{\pi}{2})$ arise as a result of mixing between states with $d$- and $p$-symmetry. This mixing, in turn, results from a desire to gain kinetic energy from hopping between the sublattices, which is not possible in the pure ZRS subspace: for this relative arrangement of the two Néel Cu sublattices, $\hat{T}_{mix}$ cannot hop a ZRS with momentum $k_x = k_y$ between neighbor Cu sites, see Fig. 2(d) of the main text. Higher-energy physics, of non-ZRS origin, then becomes relevant.

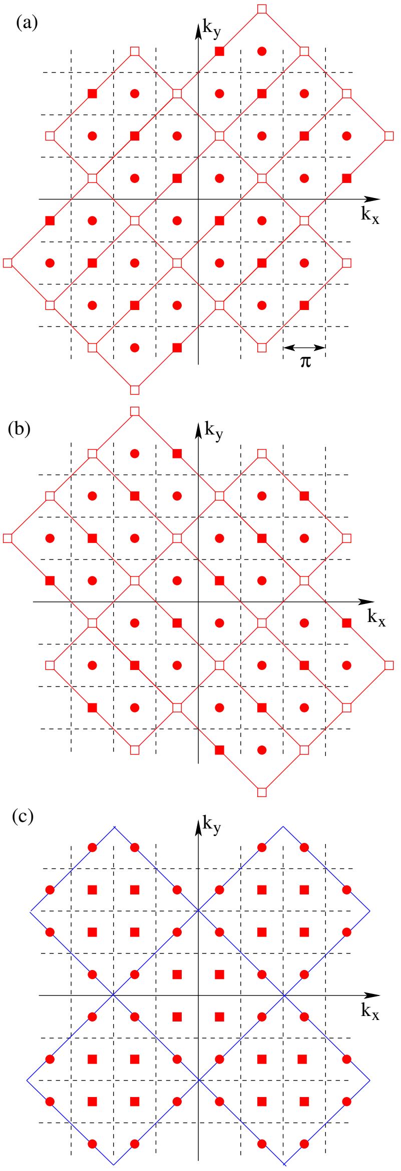


FIG. 3: The first two panels show the Brillouin zones corresponding to the two possible magnetic orders of Fig. **??**(c) and (d). The symbols mark the deep minima (full squares), displaced shallower minima (circles) and very shallow minima (empty squares). The two figures are related by a $C_4$ rotation. The third panel shows the average of these two patterns, where at each special point the deepest local minimum was selected. This pattern has a restored $C_4$ symmetry and a Brillouin zone (blue line) corresponding to one Cu site/unit cell. The pattern of deep/shallower minima is like that found experimentally.

## COMPARISON WITH ARPES DATA

The result of averaging over domains with both possible orientations is demonstrated in Fig. 3. Panel (a) shows the T-CuO Brillouin zones (red rectangles) from Fig. 2(c) of the main text, which corresponds to the magnetic order of Fig. 1(c). The symbols mark the deep minima (full squares), displaced shallower minima (circles) and very shallow minima (empty squares). Panel (b) is obtained by a $C_4$ rotation and corresponds to the magnetic order of Fig. 1(d). Their average is shown in panel (c), where the symbols now mark the lowest-energy local minimum. The resulting pattern agrees with that measured experimentally for T-CuO. The large Brillouin zones (blue squares) corresponding to a unit cell with one Cu per basis emerges naturally, as do the patterns of deep and shallower minima.

Fig. 4 shows the quasiparticle dispersion along the same contour discussed in Fig. 1 of Ref.[20] of main paper, for both magnetic orientations. Note that our results are in hole language, so to compare with their ARPES data the energies should be reversed, $E_{qp} \to -E_{qp}$. For ease of comparison, the lower panel shows the same results in this electron picture, with the symmetry points also labelled like in Ref. [20].

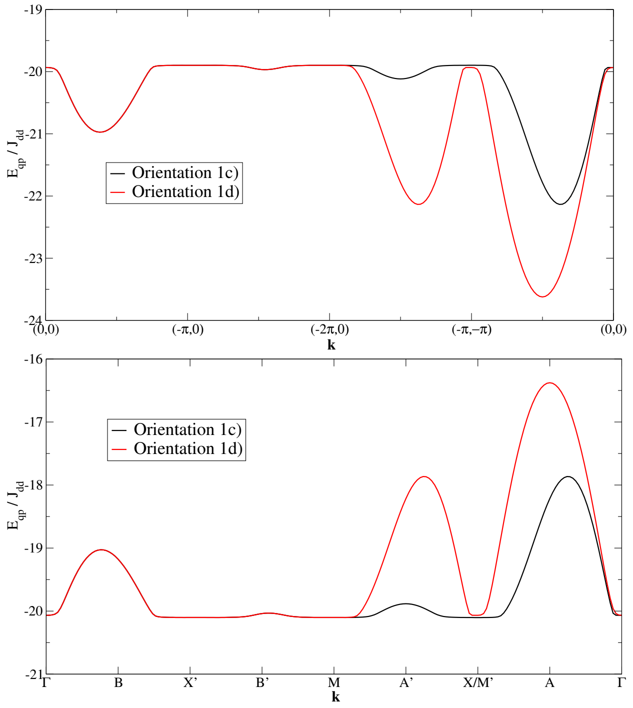


FIG. 4: Quasiparticle dispersion for the two orientations of the magnetic background, along the contour considered in Ref. [20]. Top panel shows the results in the hole picture used throughout this work, whereas the low panel shows the same results in the electron picture relevant for experiments, with further tuning of the parameters. Also, we note that the slight displacements of the shallower minima have not been observed experimentally. This may be because of the very broad widths of the quasiparticle peaks and the loss of spectral weight on one side of these points, which may mask them. In “untwinned” samples the scattering rate should be lower, which may make the observation of these displacements towards Γ more easily visible. Of course, in that case the lack of $C_4$ symmetry and existence of really shallow minima should also become visible.
